# Supplementary material for: Pressure tuning of structure, magnetic frustration and carrier conduction in Kitaev spin liquid candidate Cu$_2$IrO$_3$: X-ray, Raman, magnetic susceptibility, resistivity and first-principles analysis
Source: arXiv:2205.00966 ancillary file (2022-05-02)
Supplement: Supplementary file 1 [file Supplementary.pdf]

# Supplementary Information: Pressure tuning of structure, magnetic frustration and carrier conduction in Kitaev spin liquid candidate $Cu_2IrO_3$: X-ray, Raman, magnetic susceptibility, resistivity and first-principles analysis

Srishti Pal†,[1,*] Pallavi Malavi†,#,[1] Arijit Sinha,[2] Anzar Ali,[3] Piyush Sakrikar,[3] Boby Joseph,[4] Umesh V. Waghmare,[2] Yogesh Singh,[3] D. V. S. Muthu,[1] S. Karmakar,[5] and A. K. Sood[1]

[1]*Department of Physics, Indian Institute of Science, Bengaluru 560012, India*

[2]*Theoretical Sciences Unit, Jawaharlal Nehru Centre for Advanced Scientific Research, Bengaluru 560064, India*

[3]*Department of Physical Sciences, Indian Institute of Science Education and Research (IISER) Mohali, Knowledge City, Sector 81, Mohali 140306, India*

[4]*Elettra-Sincrotrone Trieste S.C. p. A., S.S. 14, Km 163.5 in Area Science Park, Basovizza 34149, Italy*

[5]*HP&SRPD, Bhabha Atomic Research Centre, Trombay, Mumbai 400085, India*

(Dated: May 2, 2022)

## I. X-RAY DIFFRACTION

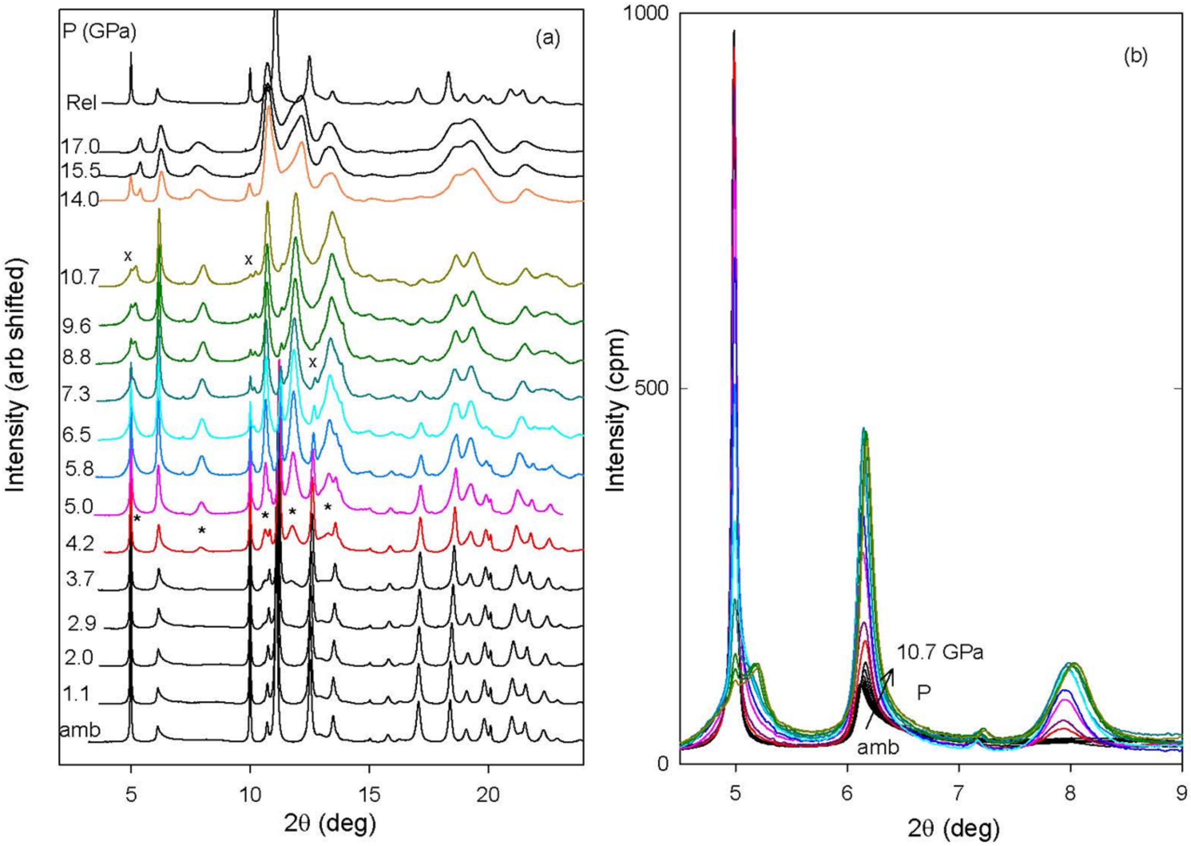


FIG. S1. (a) X-ray diffraction patterns (intensity arbitrarily shifted) of $Cu_2IrO_3$ at various high pressures from two different runs (plots up to 10.7 GPa are with MEW as PTM and displayed patterns of higher pressures are with silicone oil as PTM). (b) Plots of XRD patterns (with as obtained intensity, in counts per min) up to 10.7 GPa in the low diffraction angle range (4.5-9°).

$Cu_2IrO_3$ undergoes very sluggish structural transition, monoclinic ($C2/c$) to triclinic ($P\bar{1}$), above ~4 GPa. The transition is completed by ~15 GPa. Clear emergence of the new Bragg peaks is shown by '*' at pressure 4.2 GPa [Fig. S1(a)]. Also, much reduced Bragg peaks of the low-pressure monoclinic phase are shown by '×' at 7.3 and 10.7 GPa. Mixed phase patterns are shown in colour. The structural transition is found completely reversible, as shown in top profile at ~0.1 GPa released from 17 GPa. Figure S1(b) shows XRD patterns between $2\theta = 4.5$-9° at a few selected pressures up to 10.7 GPa. The peaks at $2\theta = 5°$ are two single Bragg peaks, characteristic of two phases. The systematic variation

of the peak intensity clearly indicates a mixed phase region; the high pressure phase grows as the low $P$ monoclinic phase intensity gets suppressed. Enhanced intensity of the 6° peak is a clear signature of heavily distorted honeycomb layer in the triclinic phase. The refined structural parameters of both the monoclinic ($C2/c$) and triclinic ($P\bar{1}$) phases at selected pressures are listed in Table S1.

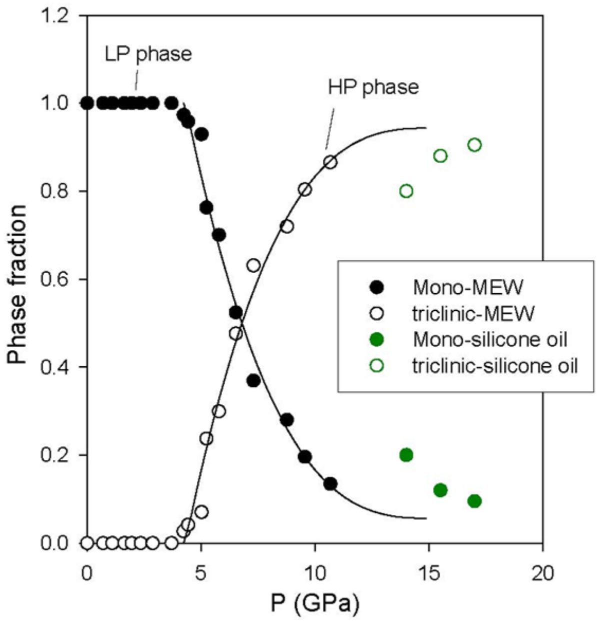


FIG. S2. Variations of phase fraction of the low $P$ monoclinic phase and the high $P$ triclinic phase with increasing pressure in two runs.

Based on the integrated intensity analysis of the low angle ($2\theta = 5°$) (002) Bragg peaks of the monoclinic and triclinic phase, we have plotted the phase fraction in the mixed phase pressure range (4-15 GPa) across the structural transition in two different pressure measurements as shown in Fig. S2. Although transition starts nearly at 4 GPa in both the measurements (run1 with 16:3:1 MEW as PTM and run2 with silicone oil as PTM), the transition is found more sluggish in case of non-hydrostatic measurement (in run2), indicated by presence of non-zero phase fraction of the low $P$ phase. However, this is only based on the low angle single peak. At higher angles, no Bragg peak corresponding to monoclinic phase is observed above 15 GPa.

Variation of unit cell volume and interlayer separation between honeycomb layers are plotted in Fig. S3. Fitting the $P - V$ data using third order Birch-Murnaghan (3BM) equation of state[1] gives the values of the bulk modulii in the low-pressure monoclinic ($C2/c$)

TABLE. S1. Structural details as extracted from the analyses of the XRD profiles at various high pressures.

| P (GPa) | Space group | Lattice constants | P (GPa) | Atom | $x$ | $y$ | $z$ | Occupancy |
|---|---|---|---|---|---|---|---|---|
| | | $a = 5.3849$ Å | | Ir1 | 0.25 | 0.079 | 0 | 0.81 |
| | | $b = 9.3252$ Å | | Cu1 | 0.25 | 0.079 | 0 | 0.19 |
| 0.7 | $C2/c$ | $c = 11.517$ Å | | Ir2 | 0.25 | 0.25 | 0.5 | 0.37 |
| | | $\beta = 99.42°$ | | Cu2 | 0.25 | 0.25 | 0.5 | 0.62 |
| | | | 0.7 | Cu3 | 0 | 0.75 | 0.25 | 1 |
| | | $a = 5.3524$ Å | | Cu4 | 0 | 0.455 | 0.25 | 1 |
| | | $b = 9.2249$ Å | | Cu5 | 0 | 0.08 | 0.25 | 1 |
| 5.8 | $C2/c$ | $c = 11.5794$ Å | | O1 | 0.949 | 0.75 | 0.09 | 1 |
| | | $\beta = 101.477°$ | | O2 | 0.94 | 0.42 | 0.078 | 1 |
| | | | | O3 | 0.932 | 0.084 | 0.091 | 1 |
| | | $a = 5.0805$ Å | | Ir1 | 0.4775 | 0.3057 | 0 | 1 |
| | | $b = 9.2341$ Å | | Ir2 | 0.5042 | 0.7904 | 0.5 | 1 |
| | | $c = 10.928$ Å | | Ir3 | 0.0296 | 0.3048 | 0.5 | 1 |
| 5.8 | $P\bar{1}$ | $\alpha = 90.731°$ | | Ir4 | -0.0267 | 0.7946 | 0 | 1 |
| | | $\beta = 100.321°$ | | Cu1 | 0.5 | 0 | 0 | 1 |
| | | $\gamma = 92.853°$ | | Cu2 | 0.5 | 0.5 | 0.5 | 1 |
| | | | | Cu3 | 0 | 0 | 0.5 | 1 |
| | | $a = 5.1403$ Å | | Cu4 | 0 | 0.5 | 0 | 1 |
| | | $b = 9.1068$ Å | | Cu5 | 0.25 | 0 | 0.25 | 1 |
| 17 | $P\bar{1}$ | $c = 10.644$ Å | | Cu6 | 0.75 | 0.48 | 0.25 | 1 |
| | | $\alpha = 91.188°$ | | Cu7 | 0.25 | 0.72 | 0.25 | 1 |
| | | $\beta = 101.51°$ | | Cu8 | 0.75 | 0.22 | 0.25 | 1 |
| | | $\gamma = 95.307°$ | 17 | Cu9 | 0.25 | 0.31 | 0.25 | 1 |
| | | | | Cu10 | 0.25 | 0.81 | 0.25 | 1 |
| | | | | O1 | 0.199 | 0 | 0.09 | 1 |
| | | | | O2 | 0.801 | 0.5 | 0.41 | 1 |
| | | | | O3 | 0.301 | 0 | 0.41 | 1 |
| | | | | O4 | 0.699 | 0.5 | 0.09 | 1 |
| | | | | O5 | 0.19 | 0.67 | 0.078 | 1 |
| | | | | O6 | 0.81 | 0.17 | 0.422 | 1 |
| | | | | O7 | 0.31 | 0.67 | 0.422 | 1 |
| | | | | O8 | 0.69 | 0.17 | 0.078 | 1 |
| | | | | O9 | 0.182 | 0.334 | 0.091 | 1 |
| | | | | O10 | 0.818 | 0.834 | 0.409 | 1 |
| | | | | O11 | 0.318 | 0.334 | 0.409 | 1 |
| | | | | O12 | 0.682 | 0.834 | 0.091 | 1 |

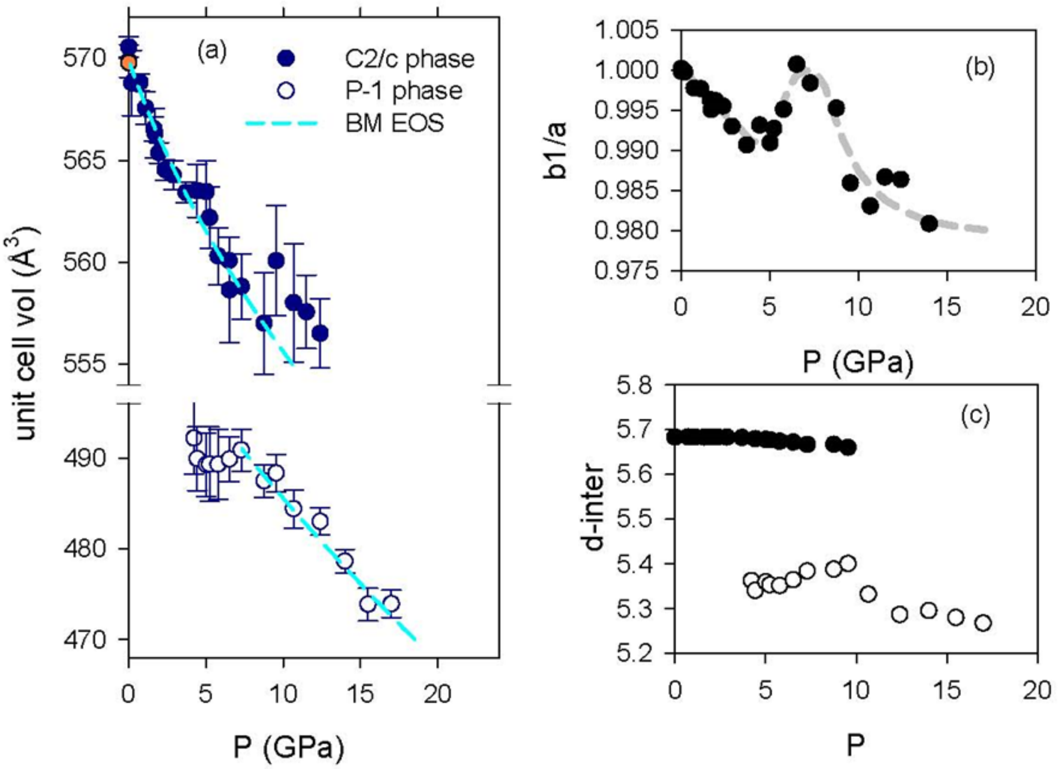


FIG. S3. (a) Unit cell volume as a function of pressure in across the structural transition. Dashed cyan lines are the Birch-Murnaghan equation of state fit for both the phases. Bulk modulii are listed in Table S2. (b) Honeycomb layer in-plane lattice parameter ratio ($b1/a$) plotted as a function of $P$. ($c$) Interlayer (honeycomb) separation $d$-inter is plotted as a function of $P$. Collapsed interlayer distance is clearly observed in the high-pressure triclinic phase.

and high-pressure triclinic ($P\bar{1}$) phases as $B_0 = 203$ (8) and 208 (13) GPa, respectively. The collapsed interlayer spacing in the high pressure triclinic phase is apparent. In the monoclinic phase, interlayer spacing remains unchanged in its stability range (up to 4 GPa), above which the spacing starts decreasing gradually. So, when we compare the interlayer spacing with in-layer lattice compression, we see that '$d$-interlayer/$a$' monotonically increases and beyond this $P$, this shows marginal declining nature as shown in Fig. S4(b). Increasing of '$d$-interlayer/$a$' results in elongation of the $IrO_6$ octahedra along the trigonal axis ($\perp$ to $ab$ plane) as shown in Fig. S4(a). This causes less compressed $IrO_6$ octahedra at higher $P$ (up to 4 GPa) and so approaches the ideal $O_h$ octahedral symmetry which is favorable for enhanced Kitaev interaction with respect to the Heisenberg exchange.

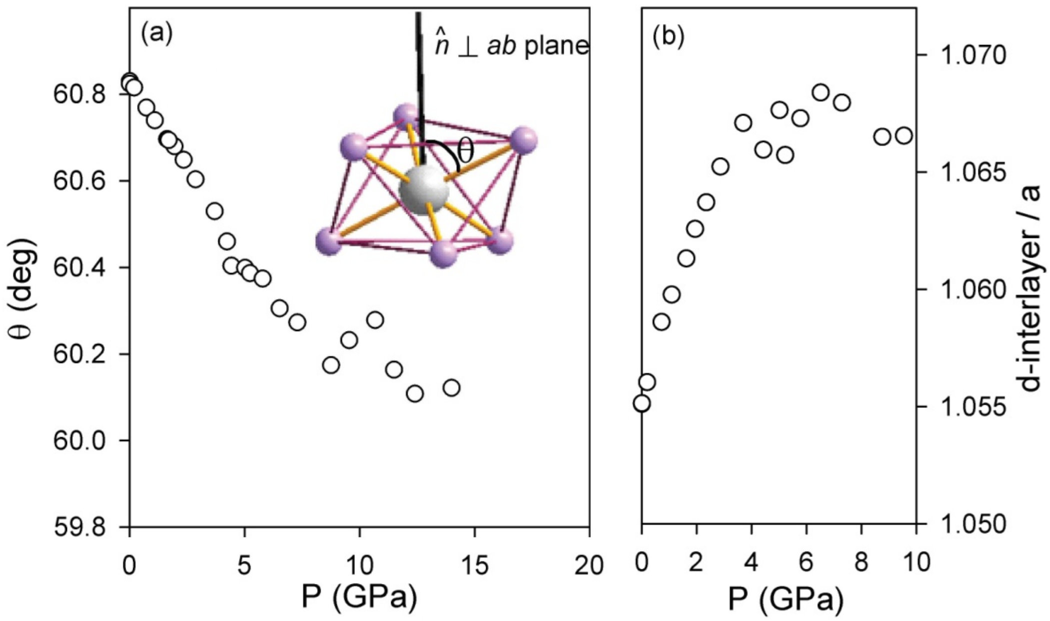


FIG. S4. (a) Pressure variation of the average azimuthal angle ($\theta$) between the Ir-O bond and normal to the $ab$-plane. A decreasing $\theta$ with increasing $P$ indicates the $IrO_6$ becomes less compressed from the $O_h$ symmetric regular $IrO_6$. (b) The ratio of interlayer separation and the Ir-Ir bond distance is also found to show $P$-induced systematic increase.

## II. RAMAN SCATTERING

The individual mode frequencies $\omega$, their $\frac{d\omega}{dP}$ values and the Grüneisen parameters $\gamma_i = \frac{B_0}{\omega}\frac{d\omega}{dP}$ ($B_0$ is the bulk modulus) are given in the Table S2.

TABLE. S2. Phonon mode frequencies, their pressure derivatives and the corresponding Grüneisen parameters for ambient and high-pressure phases of $Cu_2IrO_3$. Non-existence of modes in regions are denoted by "NE".

| Phase | $\omega (cm^{-1})$ | $\frac{d\omega}{dP} (cm^{-1}/GPa)$ I | $\frac{d\omega}{dP} (cm^{-1}/GPa)$ II | $\gamma_i = \frac{B_0}{\omega}\frac{d\omega}{dP}$ |
|---|---|---|---|---|
| Monoclinic (I) ($B_0$=203 GPa) | 83.7±0.2 | 0.0±0.02 | NE | 0.0 |
| | 93.9±0.2 | 0.2±0.03 | NE | 2.2 |
| | 509.5±0.5 | 5.5±0.1 | 2.2±0.2 | 2.2 |
| | 551.4±2.2 | 4.4±0.1 | 3.3±0.08 | 1.6 |
| | 604.7±3.4 | 4.9±0.2 | | 1.6 |
| | 659.0±2.3 | 6.8±0.2 | | 2.1 |
| Triclinic (II) ($B_0$=208 GPa) | 139.9±0.6 | NE | 1.9±0.05 | 2.8 |
| | 456.7±3.3 | NE | 2.4±0.3 | 1.1 |
| | 622.0±1.7 | NE | 3.1±0.1 | 1.0 |

## III. MAGNETIZATION M(H) PLOTS

Figure S5 shows the pressure variation of magnetic moment (∼20 mg sample) at two low temperatures. At 2.5 K, a clear non-linearity is apparent, indicating the presence of minority defect spin states in our sample.

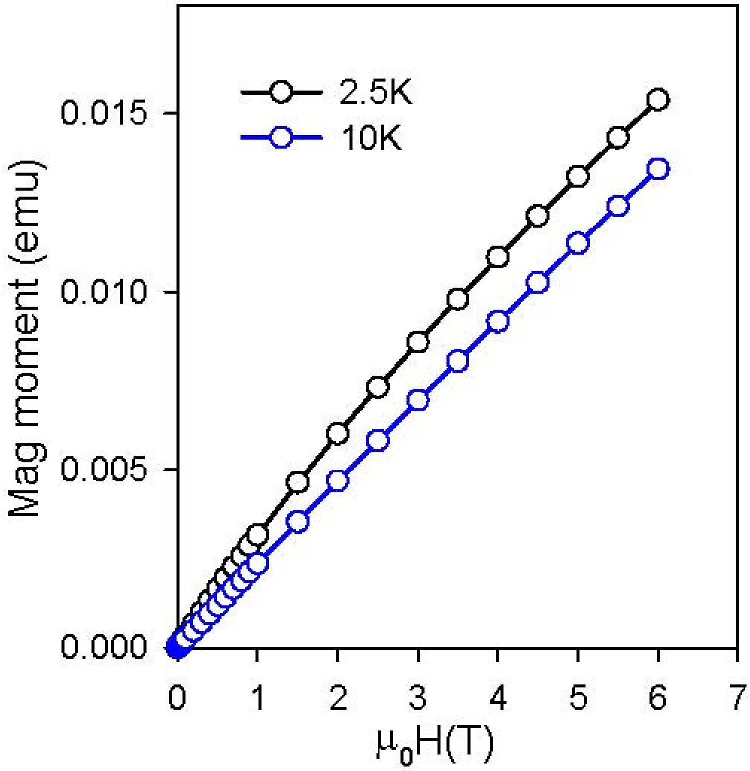


FIG. S5. $M$ $(H)$ plots for $Cu_2IrO_3$ sample at 2.5 K and 10 K.

## IV. ROOM TEMPERATURE RESISTANCE VARIATION WITH PRESSURE

Figure S6 shows the pressure variation of room temperature resistance in three successive pressure cycles. While the $R\ (P)$ variation in first and second cycle differ significantly, this remained almost unchanged in second and third cycle, indicating negligible grain boundary contribution in the pressure cycled sample.

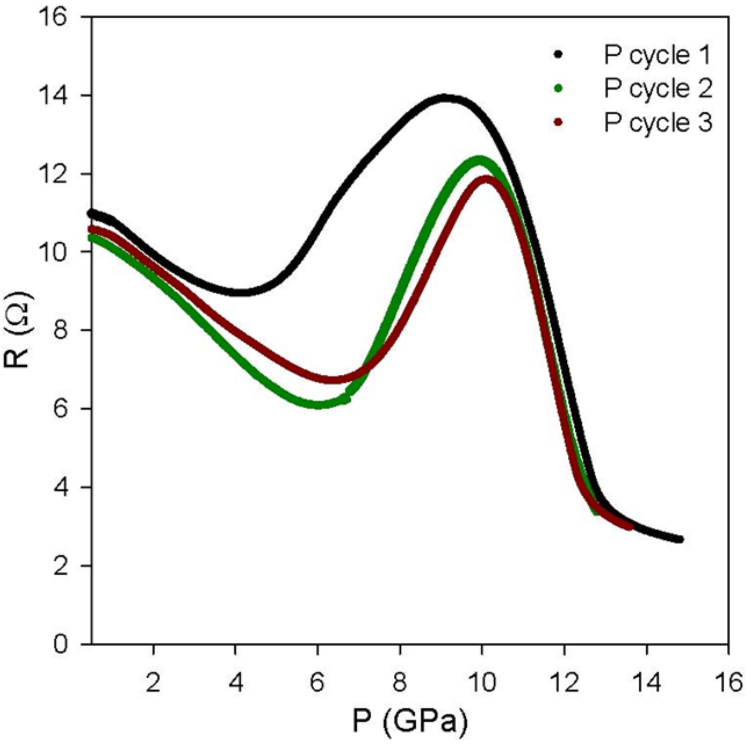


FIG. S6. Room temperature resistance in three pressure cycles up to 12 GPa.

## V. HIGH-PRESSURE RESISTANCE DATA ANALYSIS

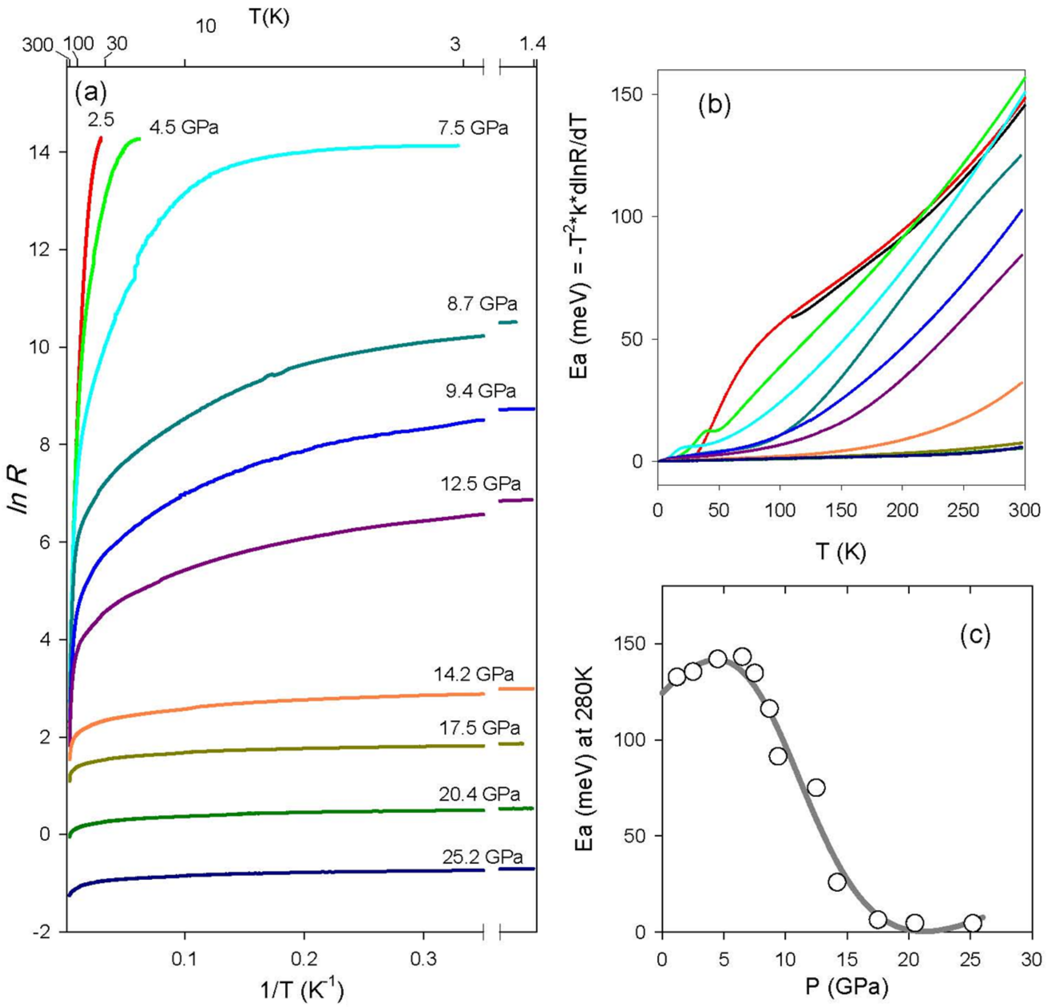


FIG. S7. (a) High pressure resistance plotted in log scale vs $1/T$ showing non-Arrhenius carrier conduction through the entire pressure range. (b) Temperature dependent activation energy (derived from the activation equation and the $dR/dT$) has been plotted for various pressures and this found to vary over the entire $T$ range. (c) As the high $T$ (near room temperature) activation energy seems more appropriate for the effective gap ($E_g = 2E_a$) determination, the Mott gap in the low-pressure phase can be estimated ~300 meV, closely matching with that of the parent compound $Na_2IrO_3$. The gap marginally changes in the low $P$ phase up to 5 GPa above which is rapidly decreases and reached ~20 meV above 15 GPa and remains unchanged at further higher $P$, a behavior similar to $Na_2IrO_3$ and $Li_2IrO_3$ above 45 GPa.

$R$ ($T$) curves have been fitted with single Mott 3D VRH term up to 4.5 GPa. This

gives the characteristic energy scale of the low $P$ monoclinic phase. In the mixed phase region (5-15 GPa), $R$ $(T)$ fits quite well with combination of two Mott 3D VRH terms with characteristic energy scales of the low $P$ phase and high $P$ triclinic phase (discussed in main text).

At higher pressures ($P > 15$ GPa), $R$ $(T)$ is fit well in combination of high $P$ phase Mott VRH term and a metallic conduction term (discussed in main text).

$$\sigma(T) = \sigma_0 exp\left[-(T_{0_{HP}}/T)^{\frac{1}{4}}\right] + \sigma_0^m\left[\frac{1}{(1 + AT + BT^2)}\right] \quad (1)$$

Figure S8 shows the plot of overall conductivity at 17.5 GPa and 25.2 GPa.

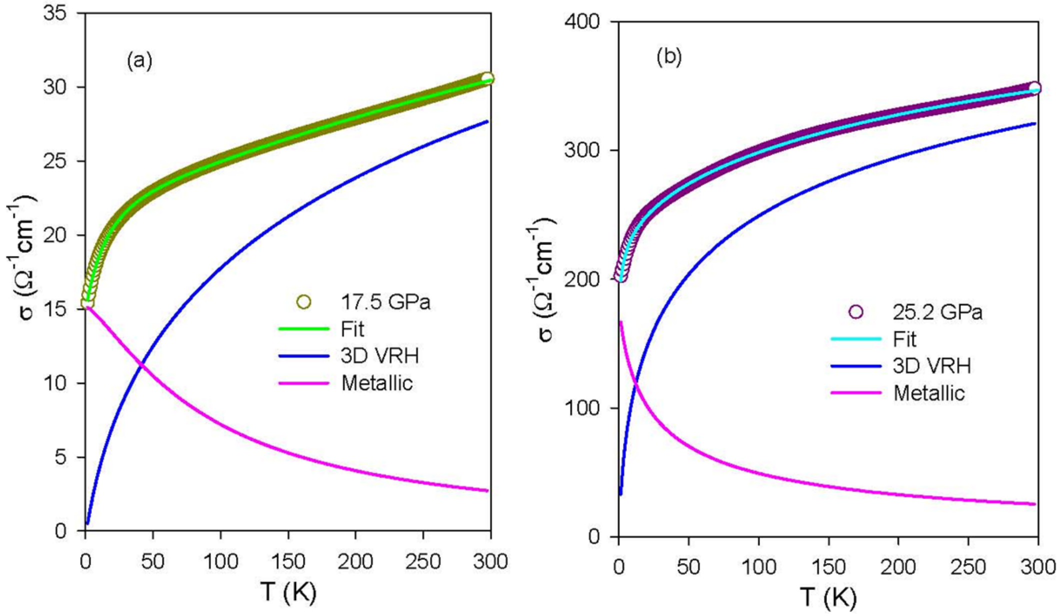


FIG. S8. The high-pressure conductivity above 15 GPa has been fitted with two contributions, (i) a Mott 3D VRH conduction and (ii) power law metallic conduction.

For 17.5 GPa, $\sigma_0 = 107\ \Omega^{-1}.\ \text{cm}^{-1}$, $T_{0_{HP}} = 915$ K, $\sigma_m = 15.1\ \Omega^{-1}.\ \text{cm}^{-1}$, $A = 9.65 \times$ 10-3 $\Omega^{-1}.\ \text{cm}^{-1}.\ \text{K}^{-1}$, and $B = 5.28 \times$ 10-5 $\Omega^{-1}.\ \text{cm}^{-1}.\ \text{K}^{-2}$.

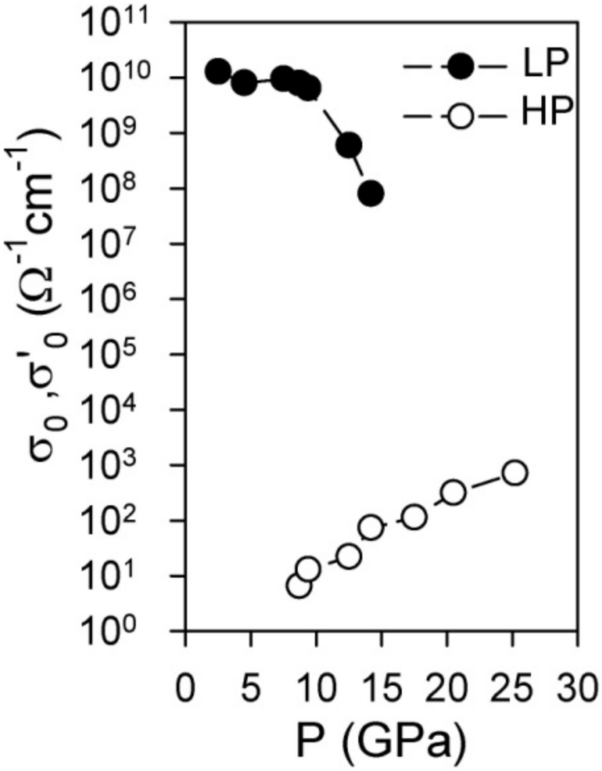


FIG. S9. Conduction coefficient of the two phases, solid circles for LP phase and open circles for HP phase.

## VI. $P = 0$ GPA, $P2_1/c$ STRUCTURE OF CIO AND BRILLOUIN ZONE

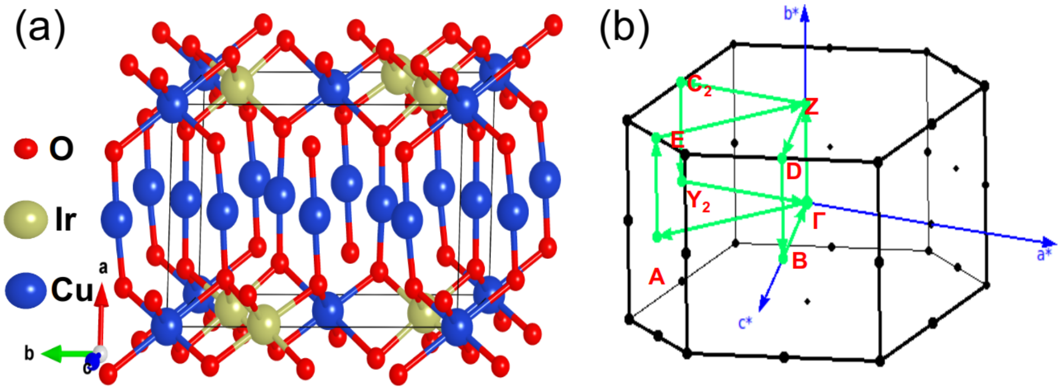


FIG. S10. (a) Conventional cell of $Cu_2IrO_3$ in $P2_1/c$ phase 2D honeycomb layers are formed by Cu-Ir atoms. (b) Brillouin zone and high-symmetry path for CIO in $P2_1/c$ phase (drawn using Xcrysden package[2]).

## VII. EVOLUTION OF CALCULATED LATTICE PARAMETERS OF $Cu_2IrO_3$ (CIO) WITH PRESSURE

Table S3 - S7 show evolution of optimized lattice parameters of CIO at pressures $P$ = 0, 5, 8, and 12 GPa using Hubbard-$U$ (6.5 eV at Cu $3d$ and 2.0 eV at Ir $5d$ orbital) and SOC interaction. Figure S11 shows displacement in atomic positions while structural transition is taking place from $P2_1/c$ structure to $P\bar{1}$ (dimerized) structure. Figure S11 reveals displacement of mainly Ir atoms in 2D honeycomb layers giving rise to dimerization in $P\bar{1}$ structure of $Cu_2IrO_3$.

TABLE. S3. Lattice parameter evolution with pressure for CIO at 0 GPa, 5 GPa, 8 GPa, and 12 GPa.

| Pressure (GPa) | Space group | $a$ (Å) | $b$ (Å) | $c$ (Å) | $\alpha$ | $\beta$ | $\gamma$ | Volume (Å$^3$) |
|---|---|---|---|---|---|---|---|---|
| 0 | $P2_1/c$ | 6.00 | 9.49 | 5.43 | 90.00 | 107.98 | 90.00 | 294 |
| 5 | $P2_1/c$ | 5.99 | 9.31 | 5.33 | 90.00 | 107.75 | 90.00 | 283 |
| 8 | $P\bar{1}$ | 5.17 | 6.02 | 9.24 | 88.60 | 87.36 | 72.74 | 274 |
| 12 | $P\bar{1}$ | 5.09 | 6.04 | 9.14 | 87.57 | 86.87 | 72.52 | 267 |

TABLE. S4. Relaxed atomic positions for CIO in 0 GPa $P2_1/c$ phase.

| Atom | Site | $x$ | $y$ | $z$ |
|---|---|---|---|---|
| Ir | 4e | 0.0087 | 0.8333 | 0.4910 |
| Cu | 2b | 0.0000 | 0.5000 | 0.5000 |
| Cu | 4e | 0.4845 | 0.1794 | 0.02160 |
| Cu | 2c | 0.5000 | 0.5000 | 0.0000 |
| O | 4e | 0.8264 | 0.5065 | 0.1076 |
| O | 4e | 0.8054 | 0.1836 | 0.1290 |
| O | 4e | 0.1619 | 0.1629 | 0.9063 |

TABLE. S5. Relaxed atomic positions for CIO at 5 GPa for $P2_1/c$ phase.

| Atom | Site | $x$ | $y$ | $z$ |
|---|---|---|---|---|
| Ir | 4e | 0.0081 | 0.8333 | 0.9930 |
| Cu | 2c | 0.0000 | 0.5000 | 0.0000 |
| Cu | 4e | 0.4858 | 0.1777 | 0.5180 |
| Cu | 2b | 0.5000 | 0.5000 | 0.5000 |
| O | 4e | 0.8233 | 0.5059 | 0.6078 |
| O | 4e | 0.8041 | 0.1812 | 0.6236 |
| O | 4e | 0.1658 | 0.1624 | 0.4057 |

TABLE. S6. Relaxed atomic positions for CIO at 8 GPa for $P\bar{1}$ phase.

| Atom | Site | $x$ | $y$ | $z$ |
|---|---|---|---|---|
| Ir | 2i | 0.9973 | 0.5078 | 0.1682 |
| Ir | 2i | 0.4893 | 0.4908 | 0.6688 |
| Cu | 1g | 0.0000 | 0.5000 | 0.5000 |
| Cu | 1e | 0.5000 | 0.5000 | 0.0000 |
| Cu | 2i | 0.4883 | 0.9813 | 0.8239 |
| Cu | 2i | 0.0138 | 0.0065 | 0.3267 |
| Cu | 1f | 0.5000 | 0.0000 | 0.5000 |
| Cu | 1a | 0.0000 | 0.0000 | 0.0000 |
| O | 2i | 0.3959 | 0.3212 | 0.4969 |
| O | 2i | 0.1025 | 0.6788 | 0.9936 |
| O | 2i | 0.3948 | 0.2940 | 0.8324 |
| O | 2i | 0.1184 | 0.6925 | 0.3187 |
| O | 2i | 0.5980 | 0.6652 | 0.8323 |
| O | 2i | 0.9126 | 0.3214 | 0.3443 |

TABLE. S7. Relaxed atomic positions for CIO at 12 GPa $P\bar{1}$ phase.

| Atom | Site | $x$ | $y$ | $z$ |
|---|---|---|---|---|
| Ir | 2i | 0.9938 | 0.5080 | 0.1686 |
| Ir | 2i | 0.4900 | 0.4899 | 0.6693 |
| Cu | 1g | 0.0000 | 0.5000 | 0.5000 |
| Cu | 1e | 0.5000 | 0.5000 | 0.0000 |
| Cu | 2i | 0.4894 | 0.9805 | 0.8236 |
| Cu | 2i | 0.0085 | 0.0059 | 0.3271 |
| Cu | 1f | 0.5000 | 0.0000 | 0.5000 |
| Cu | 1a | 0.0000 | 0.0000 | 0.0000 |
| O | 2i | 0.3973 | 0.3196 | 0.4990 |
| O | 2i | 0.1001 | 0.6808 | 0.9920 |
| O | 2i | 0.4020 | 0.2901 | 0.8372 |
| O | 2i | 0.1122 | 0.6941 | 0.3173 |
| O | 2i | 0.5977 | 0.6662 | 0.8299 |
| O | 2i | 0.9145 | 0.3175 | 0.3470 |

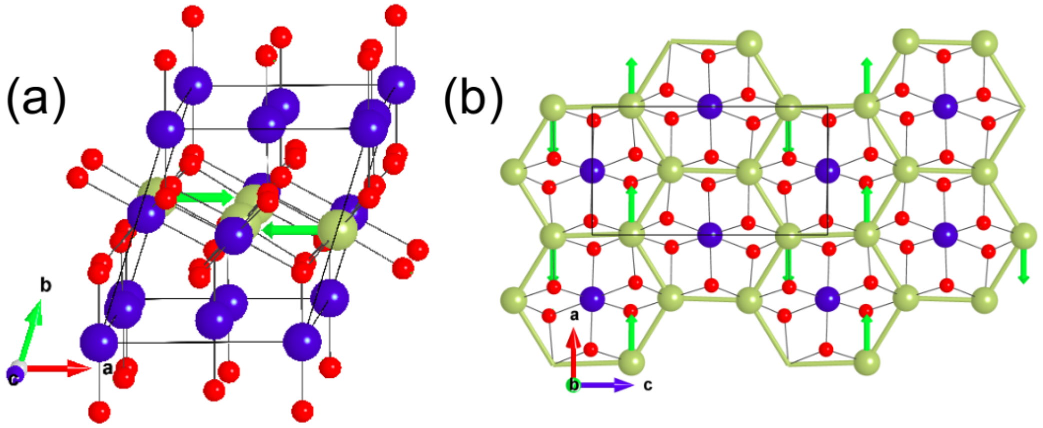


FIG. S11. During the phase transformation of CIO from $P2_1/c$ to $P\bar{1}$ (Ir-Ir bond dimerized phase) displacement of the atoms (wrt high symmetric $P2_1/c$ phase, generated using ISODISPLACE suite[3]) are denoted by green arrow, which involve displacement of Ir atoms in honey comb layer (a) side view (b) top view (Cu,O and Ir atoms are denoted by blue, red and yellow balls respectively).

## VIII. ZONE CENTRE PHONON $P2_1/c$ PHASE $P = 0$ GPA

All the frequencies of phonon modes are positive definite at Γ-point which ensures dynamical stability of CIO at 0 GPa.

TABLE. S8. CIO at 0 GPa $P2_1/c$ phase Γ-point phonon mode frequencies with mode irreducible representations, absence of unstable modes (imaginary frequencies) conclude dynamical stability of CIO at 0 GPa.

| Band index | Irreps. | Frequency ($cm^{-1}$) | Band index | Irreps. | Frequency ($cm^{-1}$) |
|---|---|---|---|---|---|
| 1, 2, 3 | - | 0 | 38 | Au | 259 |
| 4 | Au | 58 | 39 | Ag | 292 |
| 5 | Ag | 60 | 40 | Bg | 302 |
| 6 | Au | 62 | 41 | Bu | 312 |
| 7 | Ag | 66 | 42 | Au | 318 |
| 8 | Bg | 70 | 43 | Bu | 389 |
| 9 | Bu | 72 | 44 | Ag | 395 |
| 10 | Ag | 73 | 45 | Au | 406 |
| 11 | Bg | 76 | 46 | Bg | 407 |
| 12 | Au | 86 | 47 | Bg | 411 |
| 13 | Bu | 91 | 48 | Ag | 437 |
| 14 | Bu | 93 | 49 | Bu | 458 |
| 15 | Au | 97 | 50 | Ag | 461 |
| 16 | Au | 110 | 51 | Au | 467 |
| 17 | Bu | 115 | 52 | Au | 476 |
| 18 | Ag | 129 | 53 | Bu | 485 |
| 19 | Bu | 135 | 54 | Bg | 485 |
| 20 | Au | 138 | 55 | Au | 488 |
| 21 | Au | 140 | 56 | Bg | 501 |
| 22 | Bg | 142 | 57 | Bu | 501 |
| 23 | Bu | 153 | 58 | Au | 516 |
| 24 | Bg | 157 | 59 | Ag | 530 |
| 25 | Bg | 164 | 60 | Bu | 535 |
| 26 | Bu | 178 | 61 | Bg | 539 |
| 27 | Au | 184 | 62 | Ag | 541 |
| 28 | Bu | 187 | 63 | Au | 552 |
| 29 | Ag | 188 | 64 | Bg | 568 |
| 30 | Au | 200 | 65 | Bu | 591 |
| 31 | Ag | 201 | 66 | Au | 592 |
| 32 | Bg | 217 | 67 | Ag | 593 |
| 33 | Ag | 225 | 68 | Bu | 596 |
| 34 | Bu | 233 | 69 | Bg | 624 |
| 35 | Bg | 235 | 70 | Au | 637 |
| 36 | Au | 236 | 71 | Ag | 640 |
| 37 | Bu | 243 | 72 | Bu | 642 |

## IX. EVOLUTION OF PDOS WITH PRESSURE FOR LI SUBSTITUTED CIO

Pristine CIO at $P = 0$ GPa in $P2_1/c$ structure shows metallicity but experimentally it is known as an insulator with a gap ∼0.3 eV. Metallic behaviour arises due to presence of mixed valence of Ir ($Ir^{+4/+3}$) and Cu ($Cu^{+1/+2}$) (read main text for details). To remove mixed valence disorder present in 2D Cu-Ir honeycomb layers, we have substituted all the Cu atoms with Li In the optimized structure of $CuIrO_3$ (see Fig. S12). We have calculated orbital projected density electronic of states of Li substituted $Cu_2IrO_3$ at different pressures. We found electronic band gap is almost unchanged (∼0.5 eV) with change in pressure (see Fig. S13).

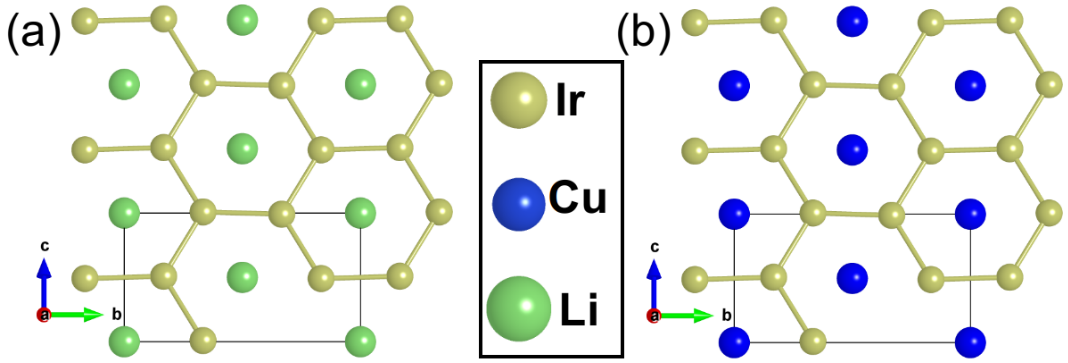


FIG. S12. (a) 2D honeycomb geometry formed by Cu-Li atoms for (a) Li substituted CIO, (b) pristine CIO in $P2_1/c$ phase (O atoms are removed for better visualization).

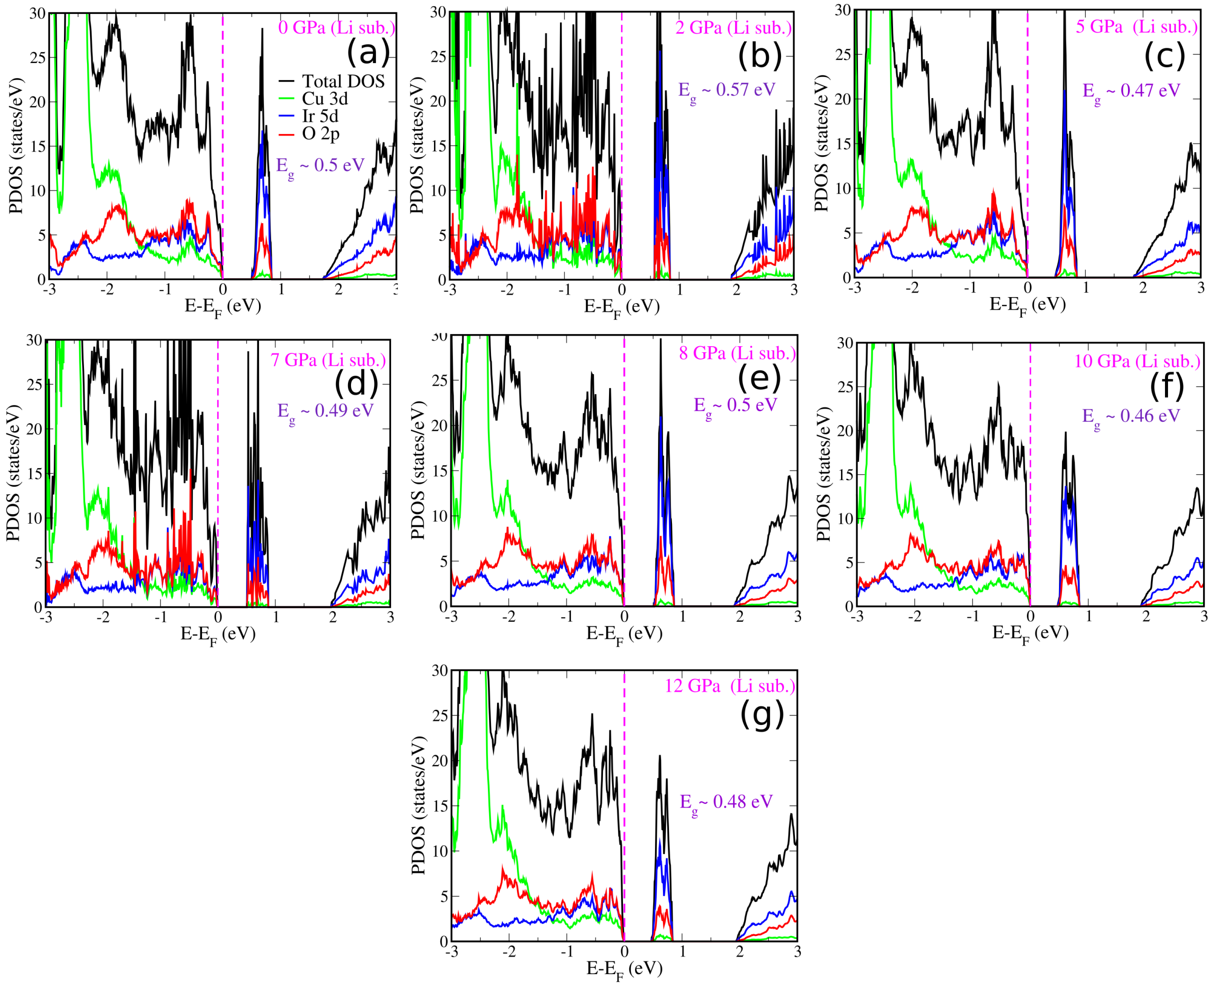


FIG. S13. Orbital projected electronic density of state for Li substituted CIO at (a) 0 GPa, (b) 2 GPa, (c) 5 GPa, (d) 7 GPa, (e) 8 GPa, (f) 10 GPa, and (g) 12 GPa which reveal band gap remains almost constant to 0.5 eV valence band maximum is constituted by Ir 5$d$, Cu 3$d$, and O 2$p$ orbitals and conduction band minimum is mainly dominated by Ir 5$d$ orbitals.

* E-mail: srishtipal@iisc.ac.in

[1] F. Birch, *J. Geophys. Res.* **91**, 4949 (1986).

[2] A. Kokalj, *J. Mol. Graph. Model.* **17**, 176 (1999).

[3] B. J. Campbell, H. T. Stokes, D. E. Tanner, and D. M. Hatch, *J. Appl. Crystallogr.* **39**, 607 (2006).
